# Supplementary material for: Bridging deep learning force fields and electronic structures with a physics-informed approach
Source: arXiv:2403.13675 ancillary file (2024-04-01)
Supplement: Supplementary file 1 [file WANDER_Supplementary_Information.pdf]

# Supplementary Information: Bridging deep learning force fields and electronic structures with a physics-informed approach

**Yubo Qi, Weiyi Gong, Qimin Yan**

## Contents

This supplementary information (SI) includes:


- **Supplementary Section 1: Atomic orbitals as the initial guess for projection**
- **Supplementary Section 2: Wannier functions before and after the localization process for finite iterations**
- **Supplementary Section 3: Structures in the training dataset**
- **Supplementary Section 4: Model for predicting vacuum level corrections**

## Supplementary Section 1: Atomic orbitals as the initial guess for projection

Fig. S1 shows the MLWFs of the ground state $MoS_2$. Tables S1 and S2 list the atomic orbitals employed to approximate the MLWFs. These orbitals are linearly independent and form a complete set, as shown in Tables S1 and S2. "Semi-localized" Wannier functions of these orbitals are used as the basis.

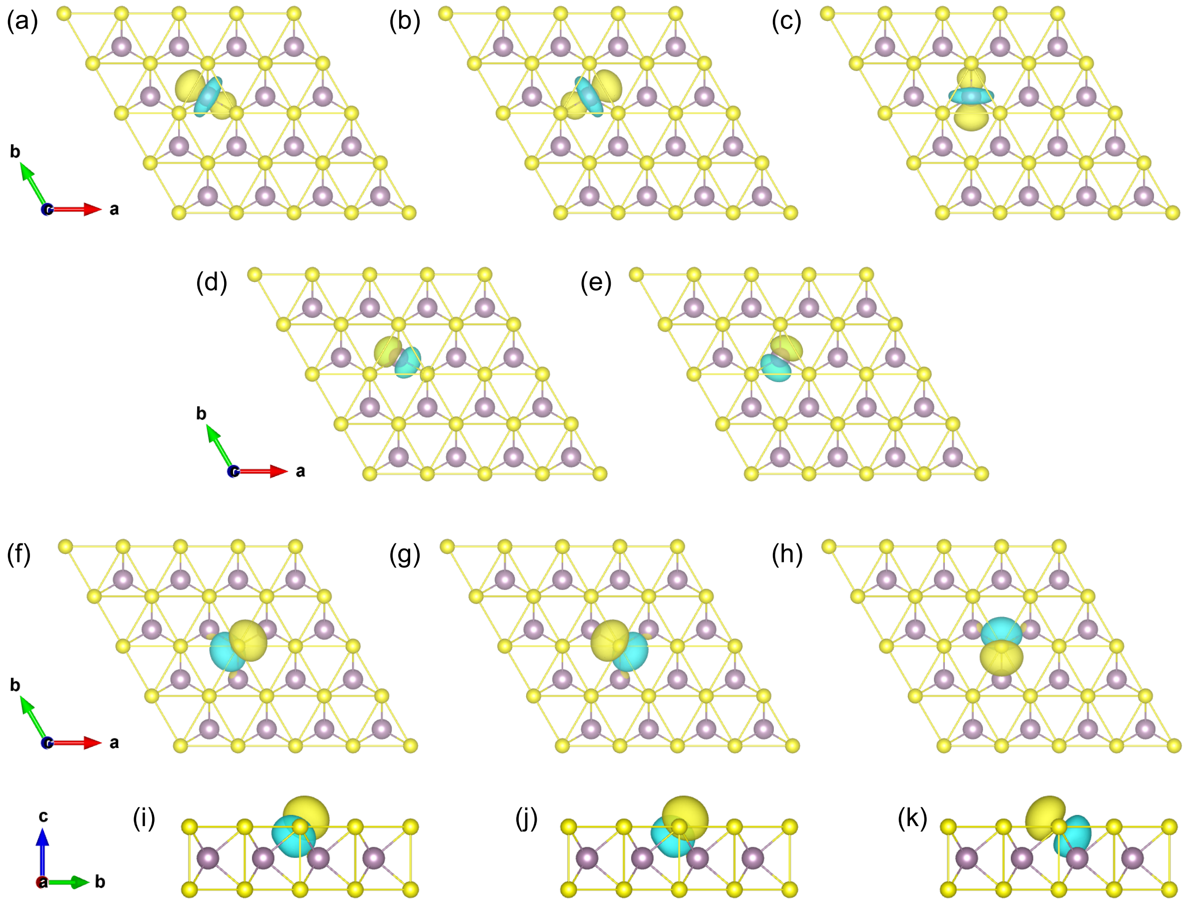


**Supplementary Figure S1. MLWFs of the ground state $MoS_2$.** (a-e) Top views of the 5 MLWFs corresponding to the *d* orbitals. (f-h) Top views of the 3 MLWFs corresponding to the *p* orbitals. (i-k) Side views of the 3 MLWFs corresponding to the *p* orbitals.

| Wannier Functions | atomic orbitals employed to approximate the MLWFs | Projections to atomic orbitals | | | | |
|---|---|---|---|---|---|---|
| | | $d_{z^2}$ | $d_{yz}$ | $d_{xz}$ | $d_{xy}$ | $d_{x^2-y^2}$ |
| $d_1$ | $d_{z^2}$ $\hat{z} =$ ( 0.866, -0.500, 0.000) | -0.500 | 0.000 | 0.000 | -0.750 | 0.433 |
| $d_2$ | $d_{z^2}$ $\hat{z} =$ (-0.866, -0.500, 0.000) | -0.500 | 0.000 | 0.000 | 0.750 | 0.433 |
| $d_3$ | $d_{z^2}$ $\hat{z} =$ ( 0.000, 1.000, 0.000) | -0.500 | 0.000 | 0.000 | 0.000 | -0.866 |
| $d_4$ | $d_{xz}$ $\hat{x} =$ (-0.866, 0.500, 0.000) | 0.000 | 0.500 | -0.866 | 0.000 | 0.000 |
| $d_5$ | $d_{yz}$ $\hat{x} =$ (-0.866, 0.500, 0.000) | 0.000 | -0.866 | -0.500 | 0.000 | 0.000 |

**Supplementary Table S1. Atomic orbitals employed to approximate the MLWFs corresponding to the *d* orbitals and their projections on atomic orbitals in Cartesian coordinates.**

| Wannier Functions | atomic orbitals employed to approximate the MLWFs | Projections to atomic orbitals | | |
|---|---|---|---|---|
| | | $d_x$ | $d_y$ | $d_z$ |
| $p_1$ | $p_z$ $\hat{z} =$ ( 0.612, 0.354, 0.707) | 0.612 | 0.354 | 0.707 |
| $p_2$ | $p_z$ $\hat{z} =$ ( -0.612, 0.354, 0.707) | -0.612 | 0.354 | 0.707 |
| $p_3$ | $p_z$ $\hat{z} =$ ( 0.000, -0.707, 0.707) | 0.000 | -0.707 | 0.707 |

**Supplementary Table S2. Atomic orbitals employed to approximate the MLWFs corresponding to the *p* orbitals and their projections on atomic orbitals in Cartesian coordinates.**

## Supplementary Section 2: Wannier functions before and after the localization process for finite iterations

Fig. S2 shows the comparison between the Wannier functions acquired from the atomic orbitals without any localization iterations and with localization with 40 iterations. The localization process changes the shapes of Wannier functions slightly.

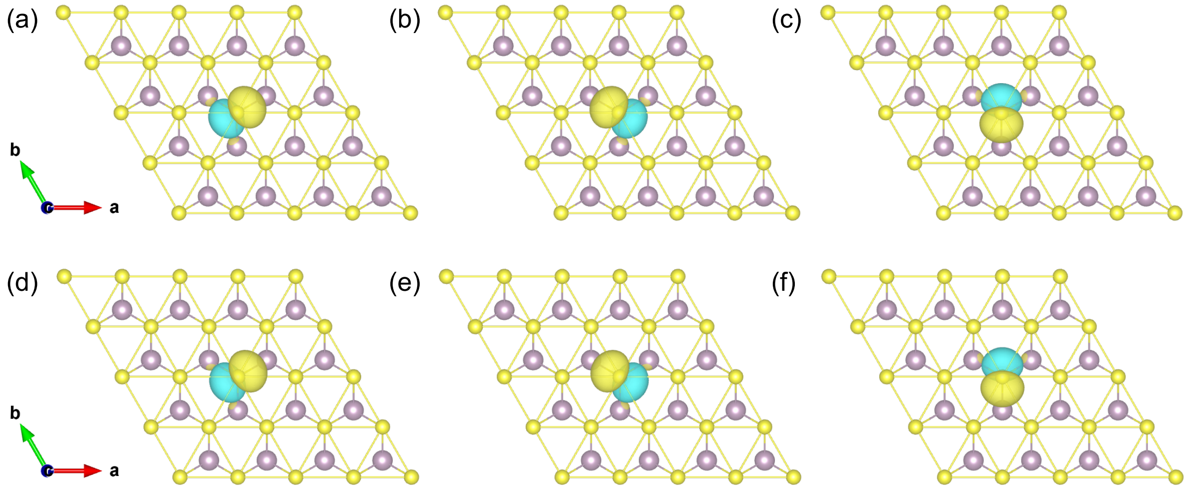


**Supplementary Figure S2. Comparison between the Wannier functions acquired from the atomic orbitals (a) without any localization iterations and (b) with localization with 40 iterations.**

## Supplementary Section 3: Structures in the training dataset

To augment the dataset for training the model, we start with the ground bilayer structure, translate the top layer with an arbitrary 3-dimensional vector, and then optimize the structure. Structures in the optimization trajectory are extracted and put into the dataset. To capture the structures with slight distortions relevant to the structure in which the two layers are related by a fixed translation, we anchor the four Mo atoms at the corners of each layer throughout the structural optimization process, as shown in Fig. S3.

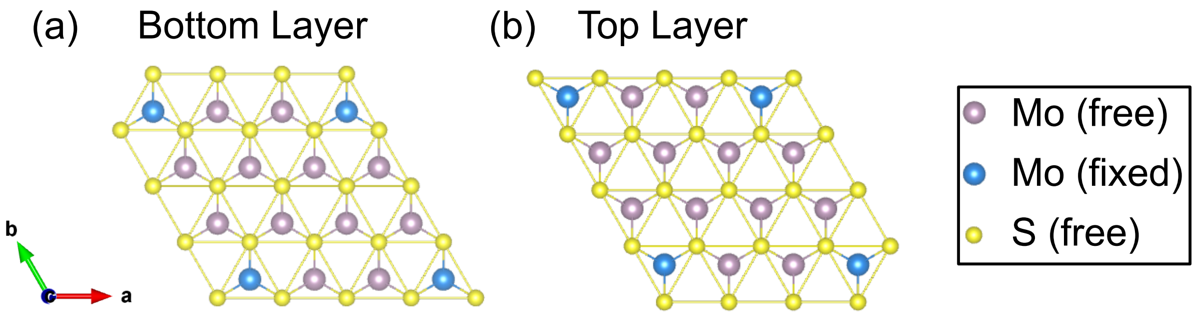


**Supplementary Figure S3. Fixed atoms during the structure optimization of the bilayer $MoS_2$ structure.**

## Supplementary Section 4: Model for predicting vacuum level corrections

Our dataset contains structures with different strains but does not include any structures with $N_{\mathrm{out}}/N_{\mathrm{in}}$ different from 1. So, the vacuum level correction term $C$ refers to the change in the vacuum level with respect to $N_{\mathrm{out}}/N_{\mathrm{in}}$ at a specific strain. We carry out DFT calculations on $MoS_2$ structures with different strains and numbers of layers. The shift in the vacuum levels can be acquired by the following two methods. First, we can refer to the energy level of the most-inner level and see how it changes in different structures. Second, we can use Wannier90 to calculate the Wannier Hamiltonian elements. We find that diagonal terms shift uniformly with structures, and such a shift in diagonal terms corresponds to the shift of the vacuum level. These two methods are equivalent. Our shallow-level machine learning model (polynomial regression) yields the following expression

$$C = \left(2.57892 - 4.56675 \times \varepsilon + 6.97391 \times \varepsilon^2 - 10.0577 \times \varepsilon^3\right) \cdot \left(\frac{N_{\mathrm{out}}}{N_{\mathrm{in}}} - 1\right)$$

The comparison between predictions and DFT results is shown in Fig. S4 (a). The model performs quite well with an R-squared value of 0.9999999. The correction term landscape as a function of $N_{\mathrm{out}}/N_{\mathrm{in}}$ and strain $\varepsilon$ is shown in Fig. S4 (b).

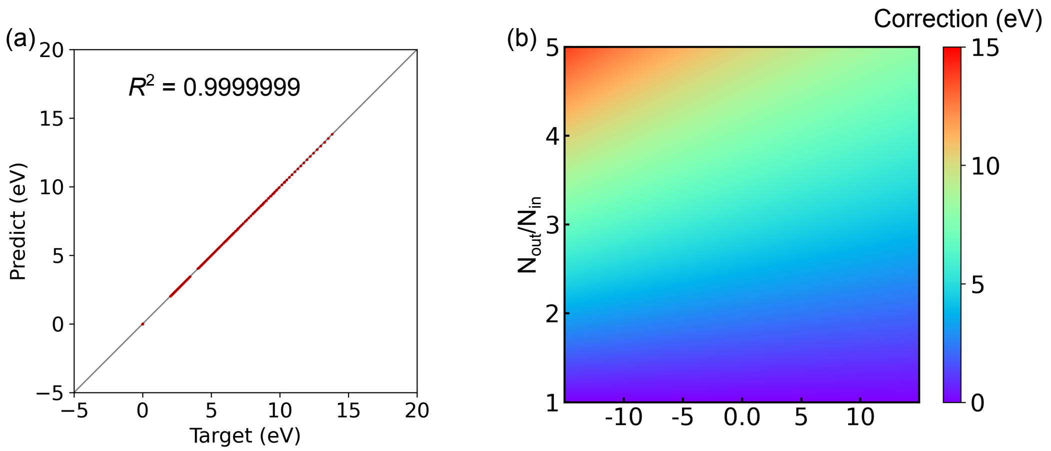


**Supplementary Figure S4. Performance of the polynomial regression model in predicting the vacuum level correction.** (a) The comparison between DFT results and model predictions. (b) The correction term as a function of atoms in the supercell and strain. The dots represent DFT results.
